# Supplementary material for: On Provable Benefits of Depth in Training Graph Convolutional Networks
Source: arXiv:2110.15174 source file (2021-10-28)
Supplement: Supplementary file 1 [file convergence_deepgcn.tex]

\section{Effect of depth on local minima in Deep GCNs} \label{supp:effect_of_depth_on_local_minima}

\subsection{Problem setups.}
Let $\mathbf{x} \in \mathbb{R}^{d_x}$ and $\mathbf{y} \in \mathbb{R}^{d_y}$ be the input and target vector, respectively. 
Let $\{(\mathbf{x}_i, \mathbf{y}_i)\}_{i=1}^N$ be a training data set of size $N$. 
Given a set of $L$ matrices $\bm{\theta} = \{ \mathbf{W}^{(\ell)} \}_{\ell=1}^L$.
Define the training data matrices as $\mathbf{X}= \{\mathbf{x}_i\}_{i=1}^N \in \mathbb{R}^{N \times d_x}$ and $\mathbf{Y}= \{\mathbf{y}_i\}_{i=1}^N \in \mathbb{R}^{N \times d_y}$. 
Let consider the squared loss function with the following training objective:
\begin{equation}\label{eq:deeper_better_obj}
    \underset{\bm{\theta}}{\text{minimize}}~F(\bm{\theta}) = \frac{1}{2} \| \widehat{\mathbf{Y}}(\bm{\theta}) - \mathbf{Y}\|_\mathrm{F}^2,~ \widehat{\mathbf{Y}}(\bm{\theta}) = \mathbf{H}^{(L)}\mathbf{W}^{(L+1)},~
    \mathbf{H}^{(\ell)} = \sigma(\mathbf{L} \mathbf{H}^{(\ell-1)} \mathbf{W}^{(\ell)}),
\end{equation}
where $[ \sigma(\mathbf{H}) ]_{i,j} = \max\{0, H_{i,j} \}$ is the coordinate-wise ReLU activation, $d_{(L+1)} = d_y$, and $d_0 = d_x$.

Let $\mathbf{\Lambda}^{\ell,k} \in \mathbb{R}^{N \times N}$ represent a diagonal matrix with diagnonal elements corresponding to the activation pattern of the $k$th unit at the $\ell$th layer over $N$ different samples as
\begin{equation}
    \Lambda_{i,i}^{\ell, k} = \begin{cases}
    1 & \text{ if } (\mathbf{L} \mathbf{H}^{(\ell-1)} \mathbf{W}^{(\ell)})_{i,k} > 0 \\ 
    0 & \text{ otherwise }  
    \end{cases}
\end{equation}
and $\mathbf{\Lambda}^\ell = \{ \mathbf{\Lambda}^{\ell,k}: ~k\in[d_{\ell-1}] \}$.

Let $\mathbf{M} \otimes \mathbf{M}^\prime$ denote the Kronecker product of matrix $\mathbf{M}$ and $\mathbf{M}^\prime$, $\Pi(\mathbf{M})$ be the orthogonal projection matrix onto the column space of a matrix $\mathbf{M}$, and $\Pi_\text{null}(\mathbf{M})$ be the orthogonal projection matrix onto the null space of a matrix $\mathbf{M}$.

\subsection{Main results}

In the following, we extend the result of the Theorem~1 of~\cite{kawaguchi2019effect} from vanilla deep non-linear model to GCN.

\begin{proposition}
Every differentiable local minimum $\bm{\theta}$ of $F(\bm{\theta})$ satisfies that
\begin{equation} \label{eq:deeper_better_minima}
    F(\bm{\theta}) = \frac{1}{2} \| \mathbf{Y} \|_\mathrm{F}^2 - \sum_{\ell\in[L+1]} \sum_{k_\ell \in [d_\ell]} \underbrace{\frac{1}{2} \left\| \Pi[N_{k_\ell}^{(\ell)} D_{k_\ell}^{(\ell)}  ] \text{vec}(\mathbf{Y}) \right\|_2^2}_{(A) \geq 0},
\end{equation}
where $D_k^{(\ell)}$ is defined as 
\begin{equation}
    \begin{aligned}
    D^{(\ell)}_k &= \begin{cases}
    \left( \prod_{j=\ell+2}^{L+1} f^{(j)}\right) f^{(\ell+1)}_k [\mathbf{L} \mathbf{H}^{(\ell-1)}] & \text{ if } \ell \in [L] \\ 
    \mathbf{I}_{d_{L+1}} \otimes \mathbf{H}^{(L)}  & \text{ if } \ell=L+1 
    \end{cases} \in \mathbb{R}^{N d_y \times d_{\ell-1}}, \\
    f^{(\ell)}_k &= \begin{cases}
    \left( (\mathbf{W}_{k,:}^{(\ell)})^\top \otimes \Lambda^{\ell-1, k} \right) \mathbf{L} \otimes \mathbf{1}_{d_{\ell-1}} & \text{ if } \ell \in [L] \\ 
    \left( (\mathbf{W}_{k,:}^{(\ell)})^\top \otimes \Lambda^{\ell-1, k} \right) & \text{ if } \ell = L+1 
    \end{cases} \in \mathbb{R}^{N d_{\ell} \times N }, \\
    f^{(\ell)} &= [f^{(\ell)}_k]_{k\in d_\ell} \in \mathbb{R}^{N d_{\ell} \times N d_{\ell-1}},
    \end{aligned}
\end{equation}
and $N_{k_\ell}^{(\ell)}$ is defined as $N_{k_\ell}^{(\ell)} = \Pi_\text{null}(\bar{Q}_{k_\ell-1}^{(\ell)})$,~$\bar{Q}_{k_\ell-1}^{(\ell)}=[[Q_{k_\ell}^{(\ell)}]_{k_\ell\in d_\ell}]_{\ell\in[L]}$,~ $Q_{k_\ell}^{(\ell)} = N_{k_\ell}^{(\ell)} D_{k_\ell}^{(\ell)}$, $\bar{Q}_0^{(\ell)} = \bar{Q}_{d_{\ell-1}}^{(\ell-1)}$, and $N_1^{(1)} = \mathbf{I}_N$.
\end{proposition}

The above proposition shows that the quality of local minima tends to improve toward the global minimum value as depth and width increase. 
To extend result from vanilla deep non-linear to GCN, we need to derive term $D^{(\ell)}_k$ for the GCN structure as defined in Eq.~\ref{eq:deeper_better_obj}. Please refer to Lemma~\ref{lemma:vec_Y_and_grad} and  Lemma~\ref{lemma:vec_Y_and_grad2} for details.

\subsection{Useful lemmas}

\begin{lemma}\label{lemma:vec_Y_and_grad}
For all $\ell \in [L]$, we have 
\begin{equation}
    \text{vec}(\widehat{\mathbf{Y}}) = D^{(\ell)} \text{vec}(\mathbf{W}^{(\ell)}),~
    \frac{\partial \text{vec}(\widehat{\mathbf{Y}})}{\partial \mathbf{W}^{(\ell)}} = D^{(\ell)},
\end{equation}
where 
\begin{equation}
    \begin{aligned}
    D^{(\ell)} &= [D^{(\ell)}_k]_{k\in d_{\ell}} \in \mathbb{R}^{N d_y \times d_{\ell} d_{\ell-1}}, \\
    D^{(\ell)}_k &= \left( \prod_{j=\ell+2}^{L+1} f^{(j)}\right) f^{(\ell+1)}_k [\mathbf{L} \mathbf{H}^{(\ell-1)}] \in \mathbb{R}^{N d_y \times d_{\ell-1}}, \\
    f^{(\ell)}_k &= \begin{cases}
    \left( (\mathbf{W}_{k,:}^{(\ell)})^\top \otimes \Lambda^{\ell-1, k} \right) \mathbf{L} \otimes \mathbf{1}_{d_{\ell-1}} & \text{ if } \ell \in [L] \\ 
    \left( (\mathbf{W}_{k,:}^{(\ell)})^\top \otimes \Lambda^{\ell-1, k} \right) & \text{ if } \ell = L+1 
    \end{cases} \in \mathbb{R}^{N d_{\ell} \times N }, \\
    f^{(\ell)} &= [f^{(\ell)}_k]_{k\in d_\ell} \in \mathbb{R}^{N d_{\ell} \times N d_{\ell-1}}
    \end{aligned}
\end{equation}
\end{lemma}
\begin{proof} [Proof of Lemma~\ref{lemma:vec_Y_and_grad}]

Recall that we have
\begin{equation}
   \widehat{\mathbf{Y}} = \mathbf{H}^{(L)}\mathbf{W}^{(L+1)},~
    \mathbf{H}^{(\ell)} = \sigma(\mathbf{L} \mathbf{H}^{(\ell-1)} \mathbf{W}^{(\ell)}),
\end{equation}

Let $\mathbf{Z}^{(\ell)}$ be the pre-activation output of the $\ell$th hidden layer as $\mathbf{Z}^{(\ell)} = \mathbf{L} \mathbf{H}^{(\ell-1)} \mathbf{W}^{(\ell)}$. 

\begin{equation}
    \begin{aligned}
    \text{vec} ( \mathbf{Z}^{(\ell)} ) 
    &= \text{vec} \left(  \sum_{k=1}^{d_{\ell-1}} \Lambda^{\ell-1, k} \mathbf{L} \mathbf{Z}^{(\ell-1)}_{:,k} \mathbf{W}_{k,:}^{(\ell)} \right) \\
    &= \sum_{k=1}^{d_{\ell-1}} \left( (\mathbf{W}_{k,:}^{(\ell)})^\top \otimes \Lambda^{\ell-1, k} \right) \text{vec}( \mathbf{L} \mathbf{Z}^{(\ell-1)}_{:,k}) \\
    &= \left[ \left( (\mathbf{W}_{k,:}^{(\ell)})^\top \otimes \Lambda^{\ell-1, k} \right) \right]_{k \in [d_{\ell-1}]} \text{vec}( \mathbf{L} \mathbf{Z}^{(\ell-1)}) \\
    &= \underbrace{\left[ \left( (\mathbf{W}_{k,:}^{(\ell)})^\top \otimes \Lambda^{\ell-1, k} \right) \right]_{k \in [d_{\ell-1}]}}_{\mathbb{R}^{N d_{\ell} \times N d_{\ell-1}}} \underbrace{[ \mathbf{L} \otimes \mathbf{I}_{d_{\ell-1}}]}_{\mathbb{R}^{N d_{\ell-1} \times N d_{\ell-1}}} \underbrace{\text{vec}(\mathbf{Z}^{(\ell-1)})}_{\mathbb{R}^{N d_{\ell-1}}} \\
    &= f^{(\ell)} \text{vec}( \mathbf{Z}^{(\ell-1)}),
    \end{aligned}
\end{equation}
where 
\begin{equation}
    \begin{aligned}
    f^{(\ell)} &= \begin{cases}
    \left[ \left( (\mathbf{W}_{k,:}^{(\ell)})^\top \otimes \Lambda^{\ell-1, k} \right) \right]_{k \in [d_{\ell-1}]} [ \mathbf{L} \otimes \mathbf{I}_{d_{\ell-1}} ] & \text{ if } \ell \in [L] \\ 
    \left[ \left( (\mathbf{W}_{k,:}^{(\ell)})^\top \otimes \Lambda^{\ell-1, k} \right) \right]_{k \in [d_{\ell-1}]} & \text{ if } \ell = L+1 
    \end{cases} \\
    &= \begin{cases}
    \left[ \left( (\mathbf{W}_{k,:}^{(\ell)})^\top \otimes \Lambda^{\ell-1, k} \right) \mathbf{L} \otimes \mathbf{1}_{d_{\ell-1}}\right]_{k \in [d_{\ell-1}]} & \text{ if } \ell \in [L] \\ 
    \left[ \left( (\mathbf{W}_{k,:}^{(\ell)})^\top \otimes \Lambda^{\ell-1, k} \right) \right]_{k \in [d_{\ell-1}]} & \text{ if } \ell = L+1 
    \end{cases}
    \end{aligned}
\end{equation}

Let further define $f^{(\ell)}_k$ for $ k\in[d_\ell]$ as
\begin{equation}
    \begin{aligned}
    f^{(\ell)}_k &= \begin{cases}
    \left( (\mathbf{W}_{k,:}^{(\ell)})^\top \otimes \Lambda^{\ell-1, k} \right) \mathbf{L} \otimes \mathbf{1}_{d_{\ell-1}} & \text{ if } \ell \in [L] \\ 
    \left( (\mathbf{W}_{k,:}^{(\ell)})^\top \otimes \Lambda^{\ell-1, k} \right) & \text{ if } \ell = L+1 
    \end{cases} \in \mathbb{R}^{N d_{\ell} \times N } ,
    \end{aligned}
\end{equation}
and $f^{(\ell)} = [f^{(\ell)}_k]_{k\in d_\ell} \in \mathbb{R}^{N d_{\ell} \times N d_{\ell-1}}$.

Then, we have 
\begin{equation}
    \begin{aligned}
    \text{vec}(\widehat{\mathbf{Y}}) 
    &= \underbrace{f^{(L+1)} \ldots f^{(\ell+1)}}_{\mathbb{R}^{N d_y \times N d_\ell}} \underbrace{\mathbf{I}_{d_\ell } \otimes [\mathbf{L} \mathbf{H}^{(\ell-1)}] }_{\mathbb{R}^{N d_\ell\times d_\ell d_{\ell-1}}} \text{vec}(\mathbf{W}^{(\ell)}) \\
    &= [D_k^{(\ell)}]_{k \in [d_{\ell}]} \text{vec}(\mathbf{W}^{(\ell)}) \\
    &= D^{(\ell )} \text{vec}(\mathbf{W}^{(\ell)})
    \end{aligned}
\end{equation}
where $D^{(\ell)}_k$ is defined as
\begin{equation}
    \begin{aligned}
    D^{(L)}_k &= (W_{k,:}^{(L+1)})^\top \otimes \mathbf{\Lambda}^{L, k} [\mathbf{L} \mathbf{H}^{(L-1)}] \\
    &= f^{(L+1)}  [\mathbf{L} \mathbf{H}^{(L-1)}] \in \mathbb{R}^{N d_y \times d_{L-1}},~
    \end{aligned}
\end{equation}
for $\ell=L$ and
% \begin{equation}
% \begin{aligned}
%     D^{(L-1)}_k &= \underbrace{\left[ \left( (\mathbf{W}_{k_L,:}^{(L+1)})^\top \otimes \Lambda^{L, k_L} \right) \right]_{k_L \in [d_L]}}_{\mathbb{R}^{N d_y \times N d_L}} 
%     \underbrace{\left[ \left( (\mathbf{W}_{k,:}^{(L)})^\top \otimes \Lambda^{L-1, k} \right) \mathbf{L} \otimes \mathbf{1}_{d_{L-1}}\right]}_{\mathbb{R}^{N d_L \times N}} \underbrace{[\mathbf{L} \mathbf{H}^{(L-2)}]}_{\mathbb{R}^{N \times d_{L-2}}} \\
%     &= f^{(L+1)} f^{(L)}_k [\mathbf{L} \mathbf{H}^{(L-2)}]
% \end{aligned}
% \end{equation}
$D^{(\ell)}_k = \left( \prod_{j=\ell+2}^{L+1} f^{(j)}\right) f^{(\ell+1)}_k [\mathbf{L} \mathbf{H}^{(\ell-1)}]$ for $\ell\in[L-1]$.

Therefore, we derive the formula of $\frac{\partial \text{vec}(\widehat{\mathbf{Y}})}{\partial \text{vec}(\mathbf{W}^{(\ell)})} \in \mathbb{R}^{N d_y \times d_\ell d_{\ell-1}}$ as
\begin{equation}
    \begin{aligned}
    \frac{\partial \text{vec}(\widehat{\mathbf{Y}})}{\partial \text{vec}(\mathbf{W}^{(\ell)})}
    &=  \frac{\partial D^{(\ell)} \text{vec}(\mathbf{W}^{(\ell)})}{\partial \text{vec}(\mathbf{W}^{(\ell)})} \\
    &= D^{(\ell)}
    \end{aligned}
\end{equation}

\end{proof}

% \begin{lemma} [Lemma~2 in \cite{kawaguchi2019effect}]
% For any block matrix $[\mathbf{A}, \mathbf{B}] \in \mathbb{R}^{n\times(d_1 + d_2)}$ with real sub-matrices $\mathbf{A} \in \mathbb{R}^{n\times d_1}$ and $\mathbf{B} \in \mathbb{R}^{n\times d_2}$ such that $\mathbf{A}^\top \mathbf{B}=0$, we have $\Pi([\mathbf{A}, \mathbf{B}]) = \Pi(\mathbf{A}) + \Pi(\mathbf{B})$.
% \end{lemma}

% \begin{lemma} [Lemma~3 in \cite{kawaguchi2019effect}]
% \end{lemma}

\begin{lemma}  \label{lemma:vec_Y_and_grad2}
For $\ell=L+1$, we have
\begin{equation}
    \text{vec}(\widehat{\mathbf{Y}}) = D^{(L+1)} \text{vec}(\mathbf{W}^{(L+1)}),~
    \frac{\partial \text{vec}(\widehat{\mathbf{Y}})}{\partial \mathbf{W}^{(L+1)}} = D^{(L+1)},
\end{equation}
where $D^{(L+1)} = (\mathbf{I}_{d_{L+1}} \otimes \mathbf{H}^{(L)} ) \in \mathbb{R}^{N d_{L+1} \times d_{L+1} d_L}$.
\end{lemma}
\begin{proof} [Proof of Lemma~\ref{lemma:vec_Y_and_grad2}]
    The proof similar to Lemma~\ref{lemma:vec_Y_and_grad}
\end{proof}
