# Supplementary material for: On Provable Benefits of Depth in Training Graph Convolutional Networks
Source: arXiv:2110.15174 source file (2021-10-28)
Supplement: Supplementary file 2 [file convergence_results.tex]

\section{Proof of Theorem~\ref{theorem:optimization}}

Although the objective function used in this paper is different from the one considered in ~\cite{oono2020optimization}, the proof is similar to the proof of Theorem~1 in~\cite{oono2020optimization} and the proof of theorem~1 in~\cite{nitanda2018functional} that we first bound 

\begin{equation}
    \begin{aligned}
    \sum_{i=1}^m \| g_\ell(\bm{x}_i) + \nabla \phi(\hat{y}_i^{(\ell-1)}, y_i) \|^2 
    &= \sum_{i=1}^m \| g_\ell(\bm{x}_i) \|^2 + \sum_{i=1}^m \| \nabla \phi(\hat{y}_i^{(\ell-1)}, y_i) \|^2 + 2 \sum_{i=1}^m \langle g_\ell(\bm{x}_i), \nabla \phi(\hat{y}_i^{(\ell-1)}, y_i) \rangle \\
    &\leq \alpha_\ell^2 \sum_{i=1}^m \|\nabla \phi(\hat{y}_i^{(\ell-1)}, y_i) \|^2
    \end{aligned}
\end{equation}

Rearrange it we have
\begin{equation}\label{eq:thm_1_proof_eq1}
    \frac{1}{2} \sum_{i=1}^m\| g_\ell(\bm{x}_i) \|^2 + \sum_{i=1}^m \langle g_\ell(\bm{x}_i), \nabla \phi(\hat{y}_i^{(\ell-1)}, y_i) \rangle \leq \frac{\alpha_\ell^2-1}{2} \sum_{i=1}^m \| \nabla \phi(\hat{y}_i^{(\ell-1)}, y_i) \|^2 
\end{equation}

By Taylor's expansion, we have for any $i\in[m]$ \textcolor{red}{cross entropy loss has bounded second order}
\begin{equation}
    \phi(\hat{y}_i^{(\ell)}, y_i) \leq \phi(\hat{y}_i^{(\ell-1)}, y_i) + \langle \nabla \phi(\hat{y}_i^{(\ell-1)}, y_i), \hat{y}_i^{(\ell)}-\hat{y}_i^{(\ell-1)} \rangle + \frac{1}{2}\| \hat{y}_i^{(\ell)}-\hat{y}_i^{(\ell-1)} \|^2
\end{equation}

By summing up both side from $i=1,\ldots,m$, we have
\begin{equation}
    \begin{aligned}
    \mathcal{R}_{m}^{ce}(f_\ell) 
    &\leq \mathcal{R}_{m}^{ce}(f_{\ell-1}) + \sum_{i=1}^m \langle \nabla \phi(\hat{y}_i^{(\ell-1)}, y_i), \hat{y}_i^{(\ell)}-\hat{y}_i^{(\ell-1)} \rangle + \frac{1}{2} \sum_{i=1}^m \| \hat{y}_i^{(\ell)}-\hat{y}_i^{(\ell-1)} \|^2 \\
    &\underset{(a)}{=} \mathcal{R}_{m}^{ce}(f_{\ell-1}) + \sum_{i=1}^m \langle \nabla \phi(\hat{y}_i^{(\ell-1)}, y_i), g_\ell(\bm{x}_i) \rangle + \frac{1}{2} \sum_{i=1}^m \| g_\ell(\bm{x}_i) \|^2 \\
    &\underset{(b)}{\leq} \mathcal{R}_{m}^{ce}(f_{\ell-1}) + \frac{\alpha_\ell^2-1}{2} \sum_{i=1}^m  \| \nabla \phi(\hat{y}_i^{(\ell-1)}, y_i) \|^2
    \end{aligned}
\end{equation}
where equality (a) is due to $\hat{y}_i^{(\ell)}-\hat{y}_i^{(\ell-1)} = o_\ell(\bm{h}_i^{(\ell)}) - o_{\ell-1}(\bm{h}_i^{(\ell-1)}) = g_\ell(\bm{x}_i)$, inequality (b) is due to Eq.~\ref{eq:thm_1_proof_eq1}.

By re-arranging it we have
\begin{equation}
     \frac{1-\alpha_\ell^2}{2} \sum_{i=1}^m \| \nabla \phi(\hat{y}_i^{(\ell-1)}, y_i) \|^2 \leq  \mathcal{R}_{m}^{ce}(f_{\ell-1}) - \mathcal{R}_{m}^{ce}(f_{\ell}) 
\end{equation}

By summing up $\ell=2,\ldots,L$, we have
\begin{equation} \label{eq:thm_1_proof_eq2}
    \sum_{\ell=2}^{L} \frac{1-\alpha_\ell^2}{2}  \sum_{i=1}^m  \| \nabla \phi(\hat{y}_i^{(\ell-1)}, y_i) \|^2 \leq \mathcal{R}_{m}^{ce}(f_{1}) - \mathcal{R}_{m}^{ce}(f_{L}) \leq \mathcal{R}_{m}^{ce}(f_{1})
\end{equation}

Since we are using cross entropy loss, by Lemma~\ref{lemma:risk_to_cross_entropy_rish}, using that \textcolor{red}{$\nabla \phi(\hat{y}_i^{(L)}, y_i) = \underset{\ell\in[L]}{\min} \nabla \phi(\hat{y}_i^{(\ell)}, y_i) $}
we have
\begin{equation} \label{eq:thm_1_proof_eq3}
    \begin{aligned}
    \sum_{\ell=2}^{L} \frac{1-\alpha_\ell^2}{2}  \sum_{i=1}^m  \| \nabla \phi(\hat{y}_i^{(\ell-1)}, y_i) \|^2 
    &\geq \Big(\sum_{\ell=2}^{L} \frac{1-\alpha_\ell^2}{2} \Big)  \sum_{i=1}^m  \| \nabla \phi(\hat{y}_i^{(L)}, y_i) \|^2 \\
    &\geq \frac{1}{1+\exp(\rho)} \Big(\sum_{\ell=2}^{L} \frac{1-\alpha_\ell^2}{2} \Big) \widehat{\mathcal{R}}_{m,\rho}(F)
    \end{aligned}
\end{equation}

By combining Eq.~\ref{eq:thm_1_proof_eq2} and Eq.~\ref{eq:thm_1_proof_eq3}, we have
\begin{equation}
    \widehat{\mathcal{R}}_{m,\rho}(F) \leq \frac{2(1+\exp(\rho))}{\sum_{\ell=2}^L (1-\alpha_\ell^2)} \mathcal{R}_{m}^{ce}(f_{1})
\end{equation}

\begin{lemma} [Lemma~2 of~\cite{oono2020optimization}, Proposition~3 in~\cite{nitanda2018functional}] \label{lemma:risk_to_cross_entropy_rish}
\begin{equation}
    \widehat{\mathcal{R}}_{m,\rho}(F) \leq \Big(1+\exp(\rho)\Big) \sum_{i=1}^m \|\nabla \phi(F(\bm{x}_i), y_i)\|
\end{equation}
\end{lemma}
