# Supplementary material for: On Provable Benefits of Depth in Training Graph Convolutional Networks
Source: arXiv:2110.15174 source file (2021-10-28)
Supplement: Supplementary file 3 [file oversmoothing_for_gcns.tex]

\begin{lemma} [Lemma 3.1 from~\cite{cai2020note}]
Let $\lambda_{\min}(\mathbf{L}_\text{aug})$ as the smallest non-zero eigenvalue of $\mathbf{L}_\text{aug} :=\mathbf{D}-\mathbf{A}$. Then we have
\begin{equation}
    E(\mathbf{L} \mathbf{H}^{(\ell)}) \leq (1-\lambda_{\min}(\mathbf{L}_\text{aug}))^2 E(\mathbf{\mathbf{H}^{(\ell)}})
\end{equation}
\end{lemma}

\begin{lemma} [Lemma 3.2 from~\cite{cai2020note}]
Let $\lambda_1(\mathbf{M})$ stands for the largest singular value of any matrix $\mathbf{M}$. Then, we have
\begin{equation}
    E(\mathbf{H}^{(\ell-1)} \mathbf{W}^{(\ell)}) \leq \lambda_1(\mathbf{W}^{(\ell)}) E(\mathbf{H}^{(\ell-1)}),
\end{equation}
\end{lemma}

\begin{lemma} [Lemma 3.3 from~\cite{cai2020note}]
Let $\sigma(\cdot)$ as ReLU or Leaky-ReLU function. Then, we have
\begin{equation}
    E(\sigma(\mathbf{H}^{(\ell-1)})) \leq E(\mathbf{H}^{(\ell-1)}),
\end{equation}
\end{lemma}

%#######################################################
%#######################################################
%#######################################################
\begin{proposition} [Theorem 3.4 from~\cite{cai2020note}]
For graph convolution operation defined as
\begin{equation}
    \mathbf{H}^{(\ell)} = \sigma(\mathbf{L} \mathbf{H}^{(\ell-1)} \mathbf{W}^{(\ell)}),
\end{equation}
Let $\lambda_{\min}(\mathbf{L}_\text{aug})$ as the smallest non-zero eigenvalue of $\mathbf{L}_\text{aug} :=\mathbf{D}-\mathbf{A}$, $\sigma(\cdot)$ as ReLU or Leaky-ReLU function, we have
\begin{equation}
    E(\mathbf{H}^{(\ell)}) \leq (1-\lambda_{\min}(\mathbf{L}_\text{aug}))^2 \lambda_1(\mathbf{W}^{(\ell)}) E(\mathbf{H}^{(\ell-1)})
\end{equation}
\end{proposition}
\begin{proof}
\begin{equation}
    \begin{aligned}
    E(\mathbf{H}^{(\ell)})
    &= E(\sigma(\mathbf{L} \mathbf{H}^{(\ell-1)} \mathbf{W}^{(\ell)})) \\
    &\leq E(\mathbf{L} \mathbf{H}^{(\ell-1)} \mathbf{W}^{(\ell)}) \\
    &\leq (1-\lambda_{\min}(\mathbf{L}_\text{aug}))^2 E(\mathbf{H}^{(\ell-1)} \mathbf{W}^{(\ell)}) \\
    &\leq (1-\lambda_{\min}(\mathbf{L}_\text{aug}))^2 \lambda_1(\mathbf{W}^{(\ell)}) E(\mathbf{H}^{(\ell-1)})
    \end{aligned}
\end{equation}
\end{proof}

%#######################################################
%#######################################################
%#######################################################

\begin{proposition}
For graph convolution operation defined as
\begin{equation}
    \mathbf{H}^{(\ell)} = \sigma(\mathbf{L} \mathbf{H}^{(\ell-1)} \mathbf{W}^{(\ell)} + \mathbf{B}^{(\ell)}),
\end{equation}
where $\mathbf{B}^{(\ell)} = \{\bm{b}^{(\ell)},\ldots,\bm{b}^{(\ell)}\} \in \mathbb{R}^{N\times d}$ is consisted by stacking $N$ bias vector $\bm{b}^{(\ell)} \in \mathbb{R}^{1\times d}$.
Let $\lambda_{\min}(\mathbf{L}_\text{aug})$ as the smallest non-zero eigenvalue of $\mathbf{L}_\text{aug} :=\mathbf{D}-\mathbf{A}$, $\sigma(\cdot)$ as ReLU or Leaky-ReLU function, we have
\begin{equation}
    E(\mathbf{H}^{(\ell)}) \leq (1-\lambda_{\min}(\mathbf{L}_\text{aug}))^2 \lambda_1(\mathbf{W}^{(\ell)}) E(\mathbf{H}^{(\ell-1)})
\end{equation}
\end{proposition}
\begin{proof}
\begin{equation}
    \begin{aligned}
    E(\mathbf{H}^{(\ell)})
    &= E(\sigma(\mathbf{L} \mathbf{H}^{(\ell-1)} \mathbf{W}^{(\ell)} + \mathbf{B}^{(\ell)})) \\
    &\leq E(\mathbf{L} \mathbf{H}^{(\ell-1)} \mathbf{W}^{(\ell)} + \mathbf{B}^{(\ell)}) \\
    % &\leq (1-\lambda_{\min}(\mathbf{L}_\text{aug}))^2 E(\mathbf{H}^{(\ell-1)} \mathbf{W}^{(\ell)}) \\
    % &\leq (1-\lambda_{\min}(\mathbf{L}_\text{aug}))^2 \lambda_1(\mathbf{W}^{(\ell)}) E(\mathbf{H}^{(\ell-1)})
    &= \frac{1}{2}\sum_{i=1}^N \sum_{j=1}^N \Big\| \Big( [\mathbf{L} \mathbf{H}^{(\ell-1)} \mathbf{W}^{(\ell)}]_i + \bm{b}^{(\ell)} \Big) - \Big( [\mathbf{L} \mathbf{H}^{(\ell-1)} \mathbf{W}^{(\ell)}]_j + \bm{b}^{(\ell)} \Big) \Big\|_2^2 \\
    &= E(\sigma(\mathbf{L} \mathbf{H}^{(\ell-1)} \mathbf{W}^{(\ell)})) \\
    &\leq (1-\lambda_{\min}(\mathbf{L}_\text{aug}))^2 \lambda_1(\mathbf{W}^{(\ell)}) E(\mathbf{H}^{(\ell-1)})
    \end{aligned}
\end{equation}
\end{proof}

\begin{remark}
Notice that by measuring the over-smoothing with Dirichlet energy, we show that graph convolution operation with bias terms also lead to over-smoothing, and the bias term will not affect the speed of over-smoothing because this bias term is shared between all nodes.
This result is different from the one as shown in the Remark 2 of~\cite{huang2020tackling} that graph convolution operation with bias does not necessary lead to over-smoothing.
\textcolor{red}{We will complement our claim by empirical evaluation.}
\end{remark}

\begin{proposition}
For graph convolution operation defined as
\begin{equation}
    \mathbf{H}^{(\ell)} = \sigma(\mathbf{L} \mathbf{H}^{(\ell-1)} \mathbf{W}^{(\ell)}) + \mathbf{H}^{(\ell-1)},
\end{equation}

\end{proposition}
