# Supplementary material for: On Provable Benefits of Depth in Training Graph Convolutional Networks
Source: arXiv:2110.15174 source file (2021-10-28)
Supplement: Supplementary file 4 [file consider_nonlinearty.tex]

In this section, we discuss the changes if non-linearity of inner-layer activation function is considered.

GCN:
\begin{lemma}\label{lemma:GCN_delta_z_5}
Let denote $\mathbf{Z}^{(\ell)}$ as the node embedding before activation function, i.e., $\mathbf{H}^{(\ell)} = \sigma(\mathbf{Z}^{(\ell)})$, and $\Delta z_{\max}^{(\ell)} \triangleq \max_i \| [\mathbf{Z}^{(\ell)} - \Tilde{\mathbf{Z}}^{(\ell)}]_{i,:} \|_2$, we have
\begin{equation}
    \Delta z_{\max}^{(\ell)} \leq \sqrt{d} B_x (\sqrt{d} B_w)^{\ell-1} \Big( \| \Delta \mathbf{W}^{(1)} \|_2 + \ldots + \| \Delta \mathbf{W}^{(\ell)} \|_2\Big)
\end{equation}
\end{lemma}

Considering non-linearity mainly affect the results where gradient computation happens. 

\begin{equation}
    \begin{aligned}
    \Delta d_{\max}^{(\ell)} 
    &= \max_i \| [\mathbf{D}^{(\ell)} - \tilde{\mathbf{D}}^{(\ell)}]_{i,:} \|_2 \\
    &= \max_i \| [\mathbf{L}^\top (\mathbf{D}^{(\ell+1)} \odot \sigma^\prime(\mathbf{Z}^{(\ell)})) [\mathbf{W}^{(\ell)}]^\top - \mathbf{L}^\top (\tilde{\mathbf{D}}^{(\ell+1) } \odot \sigma^\prime(\tilde{\mathbf{Z}}^{(\ell)})) [\tilde{\mathbf{W}}^{(\ell)}]^\top ]_{i,:}\|_2 \\
    &\leq \max_i \| [\mathbf{L}^\top (\mathbf{D}^{(\ell+1)} \odot \sigma^\prime(\mathbf{Z}^{(\ell)}) ) [\mathbf{W}^{(\ell)}]^\top - \mathbf{L}^\top (\tilde{\mathbf{D}}^{(\ell+1)} \odot \sigma^\prime(\mathbf{Z}^{(\ell)}) ) [\mathbf{W}^{(\ell)}]^\top]_{i,:} \|_2 \\
    &\quad + \max_i \| [ \mathbf{L}^\top (\tilde{\mathbf{D}}^{(\ell+1)} \odot \sigma^\prime(\mathbf{Z}^{(\ell)}) ) [\mathbf{W}^{(\ell)}]^\top - \mathbf{L}^\top (\tilde{\mathbf{D}}^{(\ell+1)} \odot \sigma^\prime(\tilde{\mathbf{Z}}^{(\ell)}) ) [\mathbf{W}^{(\ell)}]^\top ]_{i,:} \|_2 \\
    &\quad + \max_i \| [ \mathbf{L}^\top (\tilde{\mathbf{D}}^{(\ell+1)} \odot \sigma^\prime(\tilde{\mathbf{Z}}^{(\ell)}) ) [\mathbf{W}^{(\ell)}]^\top - \mathbf{L}^\top (\tilde{\mathbf{D}}^{(\ell+1)} \odot \sigma^\prime(\tilde{\mathbf{Z}}^{(\ell)}) ) [\tilde{\mathbf{W}}^{(\ell)}]^\top ]_{i,:} \\
    % ###########
    &= \max_i \| [\mathbf{L}^\top ((\mathbf{D}^{(\ell+1)} - \tilde{\mathbf{D}}^{(\ell+1)}) ) [\mathbf{W}^{(\ell)}]^\top]_{i,:} \|_2 \\
    &\quad + \max_i \| [\mathbf{L}^\top (\tilde{\mathbf{D}}^{(\ell+1)}  [\mathbf{W}^{(\ell)} - \tilde{\mathbf{W}}^{(\ell)}]^\top]_{i,:} \|_2 \\
    &\quad + \max_i \| [\mathbf{L} \tilde{\mathbf{D}}^{(\ell+1)} (\mathbf{Z}^{(\ell)} - \tilde{\mathbf{Z}}^{(\ell)}) \mathbf{W}^{(\ell)} ]_{i,:} \|_2 \\
    &\leq \sqrt{d} B_w \Delta d_{\max}^{(\ell+1)} + \sqrt{d} d_{\max}^{(\ell+1)} \|\Delta \mathbf{W}^{(\ell)}\|_2 + \sqrt{d} B_w d_{\max}^{(\ell+1)} \Delta z_{\max}^{(\ell)} 
    \end{aligned}
\end{equation}

Knowing that $d_{\max}^{(\ell+1)} \leq \frac{2}{\gamma} (\sqrt{d} B_w)^{L-\ell}$ From Lemma~\ref{lemma:gcn_G_bound_4} and Lemma~\ref{lemma:GCN_delta_z_5}, we have
\begin{equation}
   \begin{aligned}
    \sqrt{d} B_w d_{\max}^{(\ell+1)} \Delta z_{\max}^{(\ell)} 
    &\leq \frac{2}{\gamma} \sqrt{d} B_x (\sqrt{d} B_w)^{L} \Big( \| \Delta \mathbf{W}^{(1)} \|_2 + \ldots + \| \Delta \mathbf{W}^{(\ell)} \|_2\Big) \\
    &\leq \frac{2}{\gamma} \sqrt{d} B_x (\sqrt{d} B_w)^{L} \| \Delta \bm{\theta} \|_2
   \end{aligned}
\end{equation}

Plugging it back, we have
\begin{equation}
    \Delta d_{\max}^{(\ell)} \leq \sqrt{d} B_w \Delta d_{\max}^{(\ell+1)} + \sqrt{d} d_{\max}^{(\ell+1)} \|\Delta \mathbf{W}^{(\ell)}\|_2 + \frac{2}{\gamma} \sqrt{d} B_x (\sqrt{d} B_w)^{L} \| \Delta \bm{\theta} \|_2
\end{equation}

% ######################################################################
% ######################################################################
% ######################################################################

\subsection{Proof of Lemma~\ref{lemma:GCN_delta_z_5}}
By the definition of $\mathbf{Z}^{(\ell)}$, we have
\begin{equation}
    \begin{aligned}
    \mathbf{Z}^{(\ell)} - \Tilde{\mathbf{Z}}^{(\ell)} 
    &= \mathbf{L} \mathbf{H}^{(\ell-1)} \mathbf{W}^{(\ell)} -   \mathbf{L} \Tilde{\mathbf{H}}^{(\ell-1)} \Tilde{\mathbf{W}}^{(\ell)}  \\
    &= \mathbf{L} \Big( \mathbf{H}^{(\ell-1)} \mathbf{W}^{(\ell)} - \Tilde{\mathbf{H}}^{(\ell-1)} \mathbf{W}^{(\ell)} + \Tilde{\mathbf{H}}^{(\ell-1)} \mathbf{W}^{(\ell)} - \Tilde{\mathbf{H}}^{(\ell-1)} \Tilde{\mathbf{W}}^{(\ell)} \Big) \\
    &= \mathbf{L} \big( \mathbf{H}^{(\ell-1)}  - \Tilde{\mathbf{H}}^{(\ell-1)} \big) \mathbf{W}^{(\ell)}  + \mathbf{L} \Tilde{\mathbf{H}}^{(\ell-1)} \big( \mathbf{W}^{(\ell)}  - \tilde{\mathbf{W}}^{(\ell)} \big)
    \end{aligned}
\end{equation}

Then, we have
\begin{equation}
    \begin{aligned}
    \Delta z_{\max}^{(\ell)}
    &= \max_i \| [\mathbf{Z}^{(\ell)} - \Tilde{\mathbf{Z}}^{(\ell)}]_{i,:} \|_2 \\
    &\leq \sqrt{d} B_w \cdot \max_i \|[\mathbf{Z}^{(\ell-1)} - \Tilde{\mathbf{Z}}^{(\ell-1)}]_{i,:}  \|_2 + \sqrt{d} h_{\max}^{(\ell-1)} \| \Delta \mathbf{W}^{(\ell)} \|_2 \\
    &= \sqrt{d} B_w \cdot z_{\max}^{(\ell-1)} + \sqrt{d} h_{\max}^{(\ell-1)} \| \Delta \mathbf{W}^{(\ell)} \|_2 \\
    \end{aligned}
\end{equation}

By induction, we have
\begin{equation}
    \begin{aligned}
    \Delta z_{\max}^{(\ell)} 
    &\leq \sqrt{d} B_w \cdot \Delta z_{\max}^{(\ell-1)} + \sqrt{d} h_{\max}^{(\ell-1)} \| \Delta \mathbf{W}^{(\ell)} \|_2 \\
    &\underset{(a)}{\leq} \sqrt{d} B_w \cdot \Delta z_{\max}^{(\ell-1)} + \sqrt{d} B_x (\sqrt{d} B_w)^{\ell-1} \| \Delta \mathbf{W}^{(\ell)} \|_2 \\
    &\leq \sqrt{d} B_w \Big( \sqrt{d} B_w \cdot \Delta z_{\max}^{(\ell-2)} + \sqrt{d} B_x (\sqrt{d} B_w)^{\ell-2} \| \Delta \mathbf{W}^{(\ell-1)} \|_2 \Big) + \sqrt{d} B_x (\sqrt{d} B_w)^{\ell-1} \| \Delta \mathbf{W}^{(\ell)} \|_2 \\
    &=(\sqrt{d} B_w)^2  \cdot \Delta z_{\max}^{(\ell-2)} + \sqrt{d} B_x (\sqrt{d} B_w)^{\ell-1} \Big( \| \Delta \mathbf{W}^{(\ell-1)} \|_2 + \| \Delta \mathbf{W}^{(\ell)} \|_2\Big) \\
    &\leq \sqrt{d} B_x (\sqrt{d} B_w)^{\ell-1} \Big( \| \Delta \mathbf{W}^{(1)} \|_2 + \ldots + \| \Delta \mathbf{W}^{(\ell)} \|_2\Big)
    \end{aligned}
\end{equation}
where (a) is due to $h_{\max}^{(\ell-1)} \leq (\sqrt{d} B_w)^{\ell-1} B_x$
